# Supplementary material for: Near-Optimal Detection in MIMO Systems using Gibbs Sampling
Source: arXiv:0910.1463 source file (2009-10-08)
Supplement: Supplementary file 1 [file testML_proof.tex]

\subsection{Proving Lemma \ref{Lem:ML_is_true_sol}}
\label{subsec:ML_proof}
In the following we proof that the ML solution is likely to be the transmitted symbol vector.\\
%%%%% Insert LEMMA %%%%%%%%
{\bf Lemma \ref{Lem:ML_is_true_sol}}
\textit{
Let the signal-to-noise ratio be chosen such that $SNR = \eta \ln(N_T)$ where $\eta$ is a constant and define $\varsigma \triangleq N_R/N_T$. For the symbol set with the cardinality $\left|\Omega\right|=2$ we have
\[
{\text{IFF}} \ \ \frac{\varsigma \eta}{2} > 1 , \ \ {\text{then}} \ \ P_{ML} \leq N_T^{-(\varsigma \eta/2-1)},
\] where $P_{ML}$ is the probability of an error in the ML solution.
}%End of italic
\vspace{2mm}
%%%%%%%%%%%%%% Proof %%%%%%%%%%%%
\begin{proof}
Define $\tilde{\sb} \triangleq \sb - \sb_{ML}$, where $\sb$ represents the transmitted vector. We can then express $\Hb\tilde{\sb}$ as $\Ss \hs$, by introducing the matrix $\Ss \triangleq {\text{diag}}\left(\tilde{\sb}^T, \ldots, \tilde{\sb}^T \right) \in \Rbb^{N_R \times N_R N_T}$ and letting $\hs \triangleq \vec\left(\Hb\right)$ be a $N_R N_T$-dimensional column vector. Then the probability of making a decision error in the decoded sequence can be expressed as
%--- Insert equation ---
%Expr. of prob. of a sequence error - part 1
\begin{equation}
\label{EQ:P_error_ML} 
\begin{split}
& P_{EP} \\ &= P\left( \left\| \yb - \sqrt{\frac{SNR}{\sigma_s^2 N_T}}\Hb\sb \right\|^2 \geq \left\| \yb - \sqrt{\frac{SNR}{\sigma_s^2 N_T}}\Hb \sb_{ML} \right\|^2\right) \\
\\ &= P\left( \left\| \upsib \right\|^2 \geq \left\| \yb - \sqrt{\frac{SNR}{\sigma_s^2 N_T}}\Hb \tilde{\sb} \right\|^2\right) \ .
\end{split}
\end{equation}
By applying the Chernoff bound in \eqref{EQ:P_error_ML} and introducing the parameter $0 \leq \kappa \leq 1$, we get the expression given in \eqref{EQ:P_error_ML_Chernoff},
%------------- Insert equation as a FIGURE ---------------
%\begin{subequations}
\begin{figure*}[!ht]
\begin{subequations}
\label{EQ:P_error_ML_Chernoff} 
\begin{align} 
P_{EP} & \leq E\left\{e^{\frac{1}{2}\kappa\left(\left\| \upsib \right\|^2 - \left\| \upsib+\sqrt{\frac{SNR}{\sigma_s^2 N_T}} \Hb\tilde{\sb} \right\|^2 \right)} \right\} = \int{\partial \upsib \partial \hs \frac{e^{-\frac{1}{2}\upsib^T\upsib}}{\sqrt{(2\pi)^{N_R}}} \frac{e^{-\frac{1}{2}\hs^T\hs}}{\sqrt{(2\pi)^{N_R N_T}}} e^{-\frac{1}{2} \kappa \left(\upsib^T\upsib - \left\| \upsib + \sqrt{\frac{SNR}{\sigma_s^2 N_T}}\Ss \hs \right\|^2 \right)} } \\
&=  \int{\frac{\partial \upsib \partial \hs}{\sqrt{(2\pi)^{N_R(N_T+1)}}} e^{-\frac{1}{2}\left[\upsib^T, \hs^T\right] \times \As \times \left[\upsib^T, \hs^T\right]^T} } \label{EQ:Det_P_error_ML} \ ,
\end{align}
\end{subequations}
\end{figure*}%\end{subequations}
%--------------- END of FIGURE equation ------------------
where $\As \triangleq \left[ {\begin{array}{*{20}c}
   {{\mathop{\rm \Ib}\nolimits}_{N_R}} & {\kappa \sqrt{\frac{SNR}{\sigma_s^2 N_T}} \Ss}  \\
   {\kappa \sqrt{\frac{SNR}{\sigma_s^2 N_T}} \Ss^T} & {{\mathop{\rm \Ib}\nolimits}_{N_R N_T }  + \kappa \frac{SNR}{\sigma_s^2 N_T} \Ss^T\Ss}  \\
\end{array}} \right]$. If we use the fact that
\[
\int_{-\infty }^\infty{\partial {\bf x} \ e^{-\frac{1}{2}{\bf x}^T{\Sigma}^{-1}{\bf x}}} = \sqrt{(2\pi)^{N_T} \det \left({\Sigma}\right)} \ \ , \Sigma \succ 0 \ ,
\] 
and assume that $\As \succ 0$ is positive definite, we can simplify the expression of $P_{EP}$ to
%--- Insert equation ---
%Expr. of prob. of a sequence error - part 2
\begin{subequations}
\label{EQ:P_error_ML_simplified} 
\begin{align}
P_{EP} & \leq  \det \left(\As \right)^{-1/2} \\
&= \det \left(\Ib_{N_R N_T} + \kappa(1-\kappa) \frac{SNR}{\sigma_s^2 N_T} \Ss^T\Ss  \right) \label{EQ:Schur_compl} \\
&= \det \left(\Ib_{N_R N_T} + \kappa(1-\kappa) \frac{SNR}{\sigma_s^2 N_T} \left\| \tilde{\sb} \right\|^2 \Ib_{N_T} \right)^{-1/2} \\
&=  \left(1 + \kappa(1-\kappa) \frac{SNR}{\sigma_s^2 N_T} \left\| \tilde{\sb} \right\|^2\right)^{-N_R/2} \label{EQ:det_trick} \ .
\end{align}
\end{subequations}
Here we have employed the Schur complement in \eqref{EQ:Schur_compl} and in \eqref{EQ:det_trick} we use  $\det \left(\Ib + \Ab \Bb \right) = \det \left(\Ib + \Bb \Ab \right)$ along with $\Ss \Ss^T = \left\|\tilde{\sb} \right\|^2 \Ib_{N_R}$. Now if we choose $\kappa = 1/2$, which leads to the highest value for \eqref{EQ:P_error_ML_simplified}, we get
%--- Insert equation ---
\begin{equation}
P_{EP}	\leq \left( 1 + \frac{SNR}{4 \sigma_s^2 N_T} \left\| \tilde{\sb} \right\|^2 \right)^{-N_T/2} \ .
\end{equation}
In order to find the probability that the ML solution is not the transmitted sequence, we sum over all symbol settings in the sequence. For simplicity we assume that the cardinality is $\left|\Omega\right|=2$, which leads to
%--- Insert equation ---
\begin{subequations}
\begin{align}
P_{ML} &\leq \sum\limits_{i = m}^{N_T}{\binom{N_T}{m} \left( 1 + \frac{SNR}{4 \sigma_s^2 N_T }m \left\| \tilde{\sb} \right\|^2 \right)^{-\varsigma N_T/2}} \\
&=  \sum\limits_{i = m}^{N_T}{\binom{N_T}{m} \left( 1 + \frac{SNR}{2 N_T}m \right)^{-\varsigma N_T/2}} \\ & \approx \sum\limits_{i = m}^{N_T}{\binom{N_T}{m} e^{-\varsigma \cdot SNR \cdot  m/2}} \label{EQ:Approx_P_EP} = \left(1 + e^{-\varsigma \cdot SNR/2} \right)^{N_T} -1 \\
&= \left(1 + e^{-\varsigma \cdot \eta \ln(N_T)/2} \right)^{N_T} -1 \label{EQ:P_EP_second_last} \ ,
\end{align}
\end{subequations}
where the approximation in \eqref{EQ:Approx_P_EP} is valid for large $N_T$. For large $N_T$ we can further simplify the expression in \eqref{EQ:P_EP_second_last} to
%--- Insert equation ---
\begin{equation}
\begin{split}
P_{ML} &\leq \left(1 + N_T^{-\varsigma \cdot \eta/2} \right)^{N_T} -1  \\ & \approx N_T^{-\left(\varsigma \cdot \eta/2-1\right)}  \ \ {\text{for}} \ \  \varsigma \eta/2 > 1  \label{EQ:P_ML_convergence} \ .
\end{split}
\end{equation}
From \eqref{EQ:P_ML_convergence} we see that the probability of error asymptotically goes to zero as $N_T \rightarrow \infty$ when $\varsigma \eta/2 > 1$.
\end{proof}
